# Supplementary material for: Trade-off shapes diversity in eco-evolutionary dynamics
Source: arXiv:1705.10516 ancillary file (2017-05-30)
Supplement: Supplementary file 1 [file Supplementary.pdf]

# Supplementary Information

Farnoush Farahpour[1], Mohammadkarim Saeedghalati[1], Verena Brauer[2], Daniel Hoffmann[1,3,4,5]

May 30, 2017

1 Bioinformatics and Computational Biophysics, Faculty of Biology, University of Duisburg-Essen, Essen, Germany

2 Biofilm Center, University of Duisburg-Essen, Essen, Germany

3 Center for Medical Biotechnology, University of Duisburg-Essen, Essen, Germany

4 Center for Computational Sciences and Simulation, University of Duisburg-Essen, Essen, Germany

5 Center for Water and Environmental Research, University of Duisburg-Essen, Essen, Germany

## I Species and strains

In literature there is no unique definition of species [1]. The ambiguity of the species concept is more severe in asexual population [1,2]. Here we use phylogenetic tree to define and classify species based on the point of divergence from a common ancestor (See [2] for discussion on pros and cons of this definition). Each branch rooted from a point of divergence in phylogenetic tree is counted as an individual species when it has endured more than $5 \times 10^4$generations considering all of its sub branches. Otherwise they are counted as the strains of their parents.

## II Trade-off function

Trade-off function used in this paper (Eq. 2 in manuscript) maps competitive ability of species to a replication rate in the range $[0, 1]$. Its functionality (by changing the exponent) allows us to study effect of the form of trade-off (convex,concave and linear) on evolutionary process.

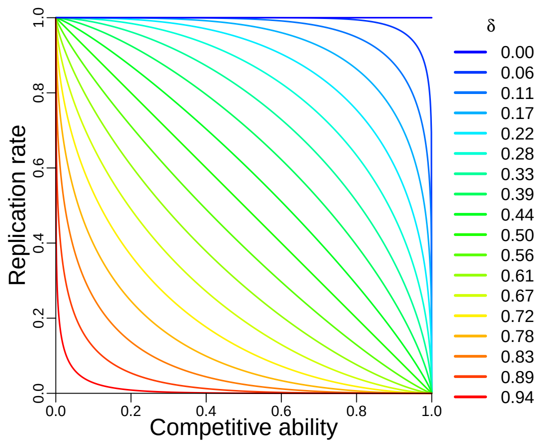


Figure 1: Trade-off functions

## III Generalized Lotka–Volterra equation

The mean-field equation equivalent to the population dynamics of the agent-based model introduced in the manuscript is a competitive generalized Lotka-Volterra equation. To show this we start from the main equation of population dynamics for our model:

$$\dot{x}_i = r_i x_i (1 - \sum x_j) + \sum r_i x_i I_{ij} x_j - \sum r_j x_j I_{ji} x_i$$

In which $x_i = \frac{n_i}{N_s}$ is the relative abundance or probability of finding species $i$ in the system. The first term in this equation shows the increase in population of species $i$ when it produces an offspring and is able to find an empty space in the system. The second term shows the increase in population of $i$ when after reproduction, its offspring is able to invade another species and the last term shows the decrease in its population due to invasion of offspring of other species. We can rewrite the equation as follows:

$$\begin{aligned}
\dot{x}_i &= x_i(r_i - \sum (r_i - r_i I_{ij} + r_j I_{ji}) x_j) \\
&= x_i(r_i - \sum (r_i(1 - I_{ij}) + r_j I_{ji}) x_j) \\
&= x_i(r_i - \sum (r_i + r_j) I_{ji} x_j) \\
&= x_i(r_i + \sum A_{ij} x_j)
\end{aligned}$$

In which we used $1 - I_{ij} = I_{ji}$. The last equation is the generalized Lotka–Volterra equation. $A$ is the community matrix and its elements $A_{ij} = -(r_i + r_j) I_{ji}$ are always negative which means that our species are in direct competition with one another. In this derivation we didn't consider the death rate or attributed lifespan of species and it can fit best with the result of $\lambda = \infty$.

## IV Classical multi-dimensional scaling (CMDS)

An MDS algorithm aims to place each object of a group in N-dimensional space such that the between-object distances are preserved as well as possible. They are usually used in information visualization, in particular to display the information contained in a distance matrix. The decision about number of dimensions N can be done by looking at the eigenvalues of factor analysis. Here we used function *cmdscale* of R package (version 3.3.0) to project our trait space into 2D plots. The distance measure is Euclidean distance.

In very early stage of evolution (Fig. 2-top) that species are very similar, 2 dimension is not sufficient to project them but when speciation and evolutionary branching occur (Fig. 2-bottom) it is more and more likely to project the trait space to 2D. This is clear in by looking at eigenvalues.

Fig. 3 shows Percentage of Variation Explained by the first two coordinates versus time for one simulation.

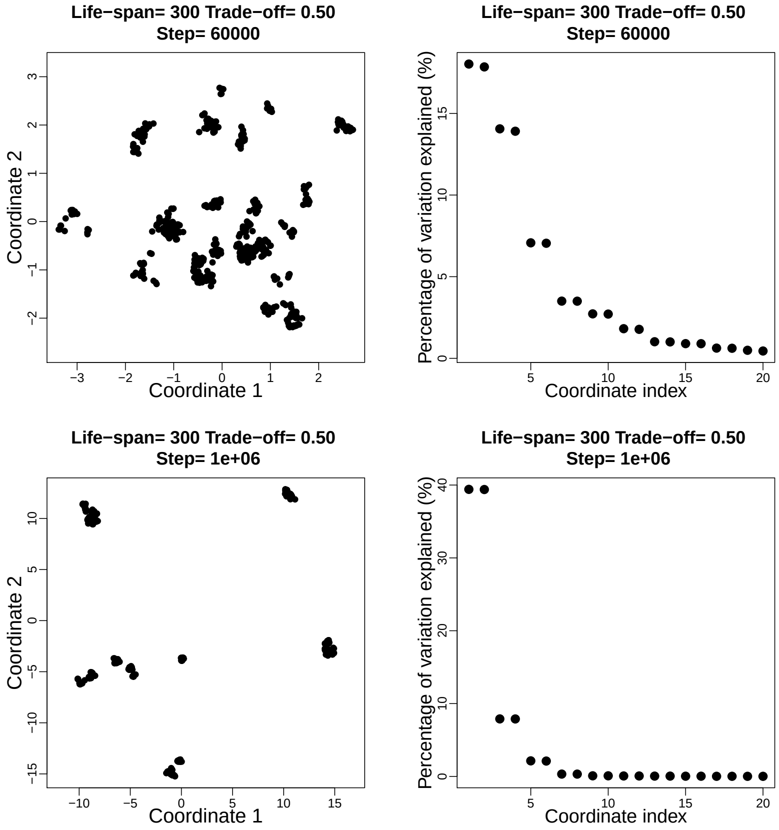


Figure 2: Top-left: Trait space at generation $6 \times 10^4$ projected into 2 dimensions using CMDS. Top-right: Percentage of variation explained by eigenvectors (correspond to the first 20 eigenvalues) of factor analysis. Here the first two eigenvectors explain around 36% of variation. Bottom: The same as the top but for generation $1 \times 10^6$. Here the first two eigenvectors explain around 78% of variation. Simulation is done with $\delta = 0.5$, $\lambda = 300$, $\mu = 0.001$ and $m = 0.02$.

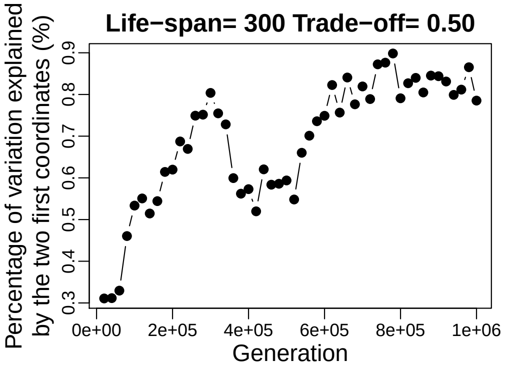


Figure 3: Percentage of variation explained by the first two coordinates versus time for one simulation. Simulation is done with $\delta = 0.5$, $\lambda = 300$, $\mu = 0.001$ and $m = 0.02$.

# V Distribution of species and strains in trait space

One way to see how species and strains are distributed over trait space is to look at the minimum spanning tree (MST) of traits in trait space. For a hierarchical structure, big edges appear between clusters or modules and small edges connect the nodes inside each cluster (Fig. 4-left). We plotted the lengths of the sorted edges of MST versus their ranks (Fig. 4-right) for 500 snapshot of simulations with $\delta = 0.5$, $\lambda = 300$, $\mu = 0.001$ and $m = 0.02$. From this plot we see that there is two clearly different scales in the size (Note the logarithmic scale of the plot). $R_1$is a representative value for the size of clusters (distance between strains of one typical species) and $R_2$ is a representative value for the size of the trait space (typical distance between different species). $N$ could be considered as a representative value for the number of distinct clusters (species) in the system.

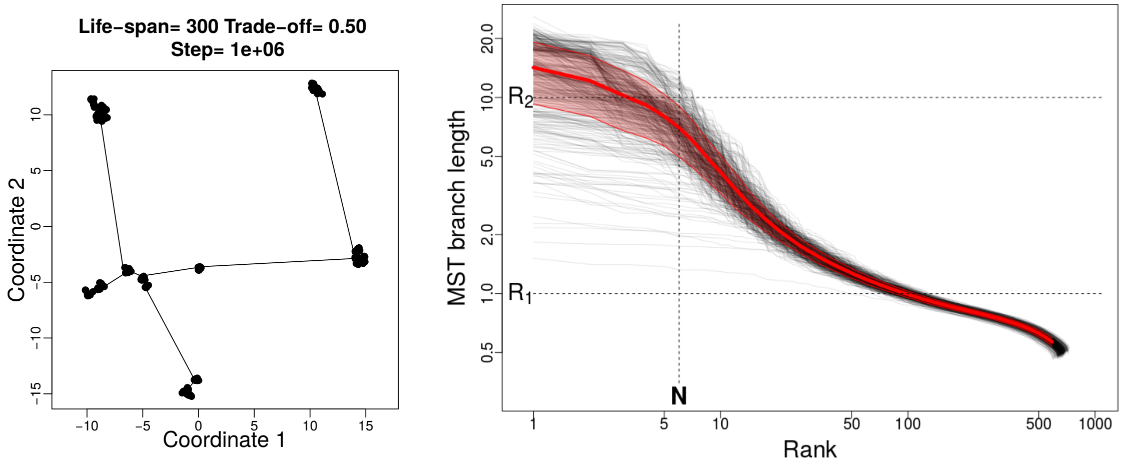


Figure 4: Left: minimum spanning tree (MST) of a typical snapshot of the simulation for $\delta = 0.5$, $\lambda = 300$, $\mu = 0.001$ and $m = 0.02$. This community of this snapshot consists of 667 strains. Right: gray curves show the sorted length of the edges of MST versus their ranks for 500 snapshots of a system with the aforementioned parameters. Red curve shows the average of all curves and the red shaded area show the standard deviation of them.

# VI Diversity indexes and parameters of dynamics

No Diversity index is sufficient to describe complete characteristics of a community. For example richness, i.e. number of species, has no information about the distribution of population among species. Evenness or equivalently Shannon entropy takes into account this distribution but has no information about the diversity of the trait of species, i.e. how diverse is a system in functionality of its species. Functional diversity indexes focus on this aspect but none of them is comprehensive to comprise all information about properties of trait space [3]. Information about density of species over resources, rate of extinction and emergence and interaction of species should be also considered to assay the dynamics of a community comprehensively.

# A Diversity over time

Next plots show how a typical diversity index changes over time. Note that evolutionary collapses (mass extinctions) occasionally occur.

Fig. 5 shows one of the indexes (Size of Minimum Spanning Tree (SMST)) over time for different trade-offs but same lifespan in each plot. Fig. 6 shows the same index (SMST) over time for different lifespans but same trade-off in each plot.

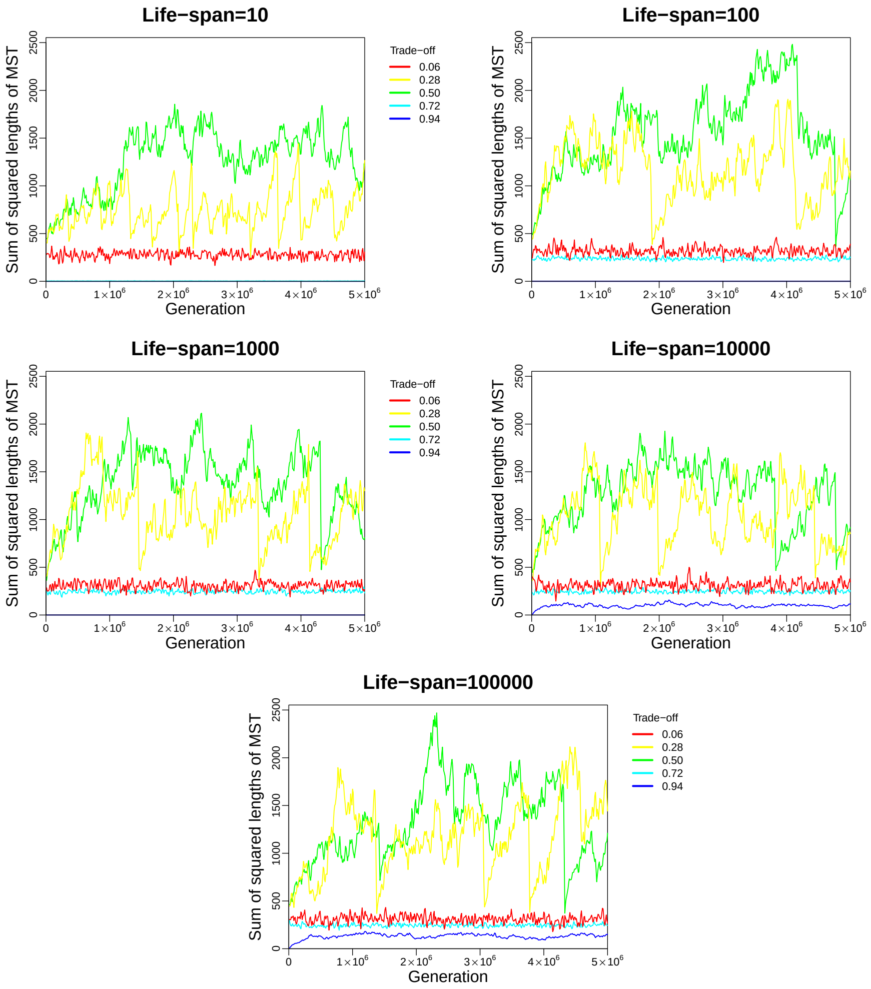


Figure 5: Each plot shows how SMST changes over generations for simulations with fixed lifespan but different trade-offs. For very strong trade-offs diverse strategies can not be adopted. For very weak trade-offs diverse strategies can emerge easily but among them extreme strategies (Darwinian Daemons) very fast dominate and diversity decreases. The most diverse communities are generated in moderate trade-offs. Very short lifespans prevent increase in diversity, specially for strong trade-offs. Simulations are done with $\mu = 0.001$ and $m = 0.02$.

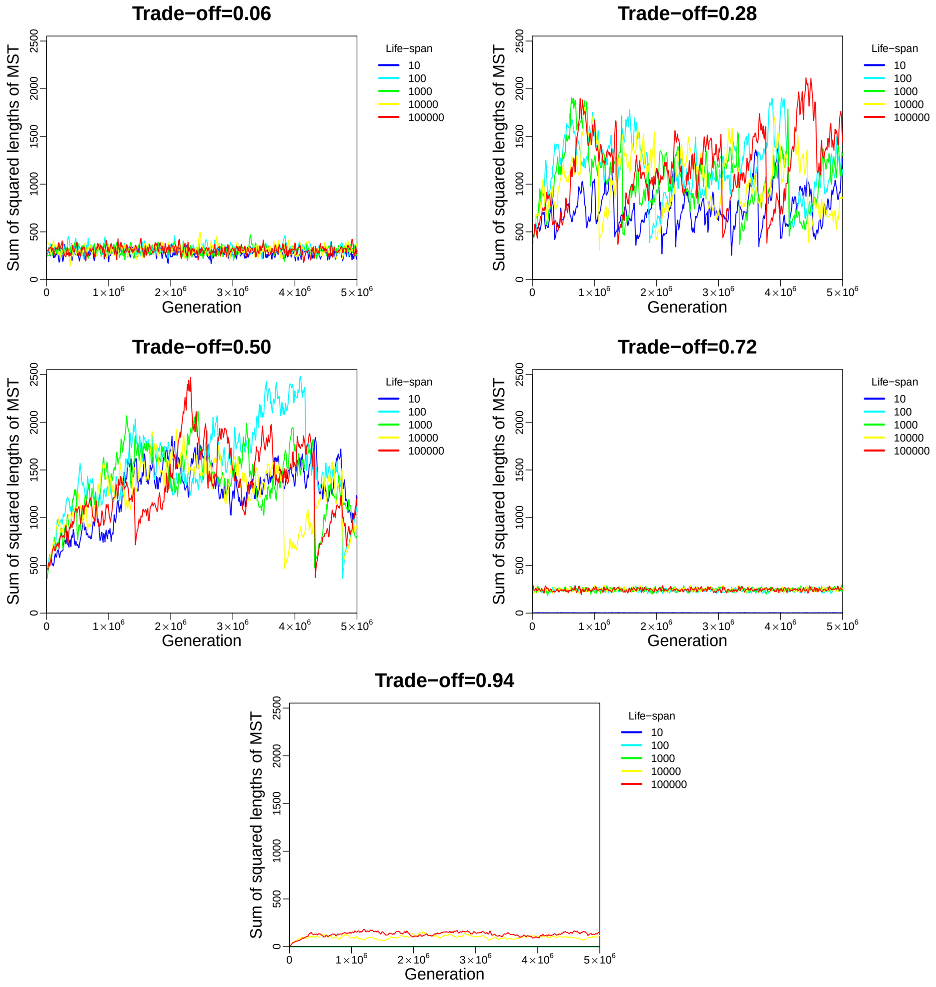


Figure 6: Each plot shows how SMST changes over generations for simulations with fixed trade-off but different lifespans. lifespan has not a big effect for weak and moderate trade-offs but for strong trade-offs, short lifespans yield to complete mass extinction. Simulations are done with $\mu = 0.001$ and $m = 0.02$.

# B Diversity indexes and parameters of dynamics for different trade-offs and lifespans

In Fig. 2 of the manuscript we have used normalized values of “richness”, “Shannon entropy”, “standard deviation of Reproduction rate”, “maximum distance in trait space”, “standard deviation of Interaction rates”, “sum of squared lengths of minimum spanning tree of trait space”, “functional diversity indexes, i.e functional dispersion, Rao index and functional evenness (all in two versions, with and without abundance)” and “strength of cycles” to compute an average as a descriptive dimensionless parameter for different regions. Although that plot can give a general idea about different behavior of communities with different $\delta$ and $\lambda$, but details of diversity indexes must be considered carefully. In Fig. 7 some of the most important parameters measured in our simulations to evaluate the community state are reported. Plots show the parameters for different trade-offs and lifespans. The Index values are averaged over $5 \times 10^6$ Generations.

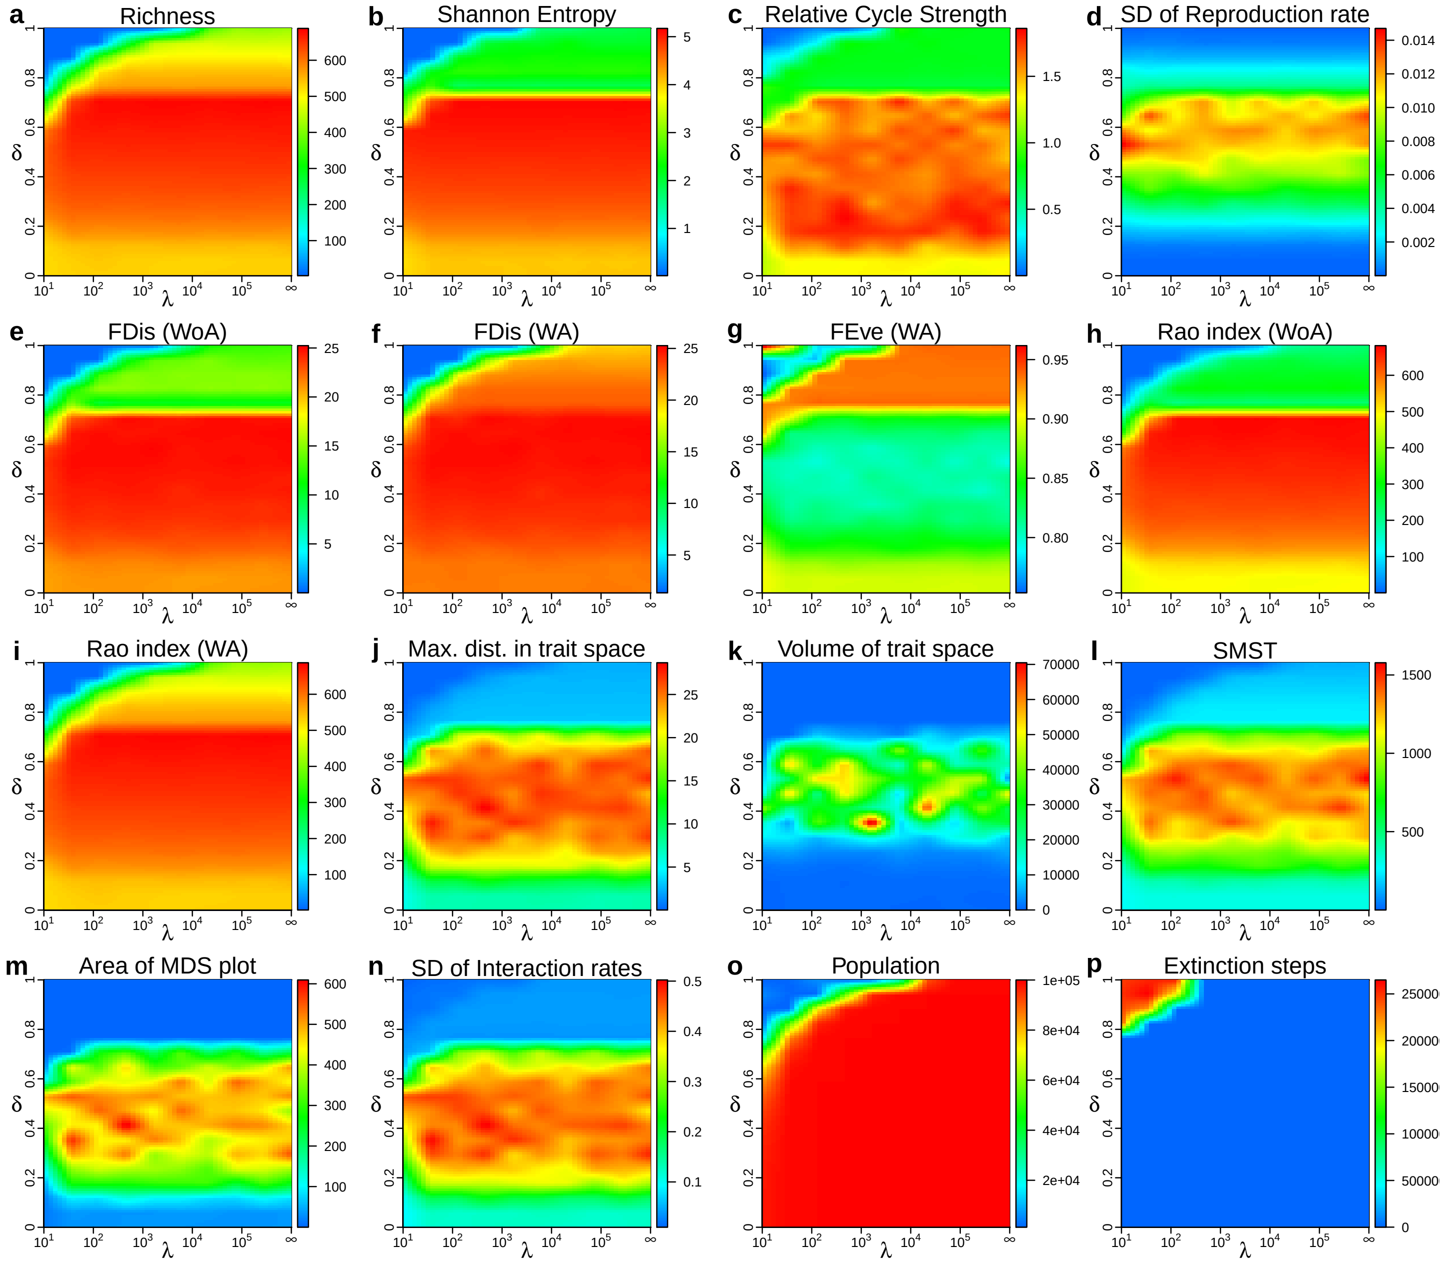


Figure 7: a) **Richness**: Number of different strains in community. b) **Shannon entropy**: which is a measure of evenness in strain population. c) **Relative Strength of cycles** of size 3 compared to random networks. (see SI-6) d) **Standard deviation of reproduction rates** as a measure of diversity in reproduction strategy. e) **Functional dispersion** (FDis, without using the abundance vector): measures the mean distance of individual strains in trait space to their centroid (dbFD function in FD package, version 1.0-12, in R) f) **Functional dispersion** (FDis, using the abundance vector): measures the mean distance of individual strains (weighted by abundance vector) in trait space to their centroid (dbFD function in FD package, version 1.0-12, in R) g) **Functional evenness** (FEve, using the abundance vector): quantifies functional evenness and is higher when species are spread homogeneously in trait space. When disruptive selection produces colonies of localized strains in trait space this index decreases (dbFD function in FD package, version 1.0-12, in R). h) **Rao's quadratic entropy** (without using the abundance vector): measures mean functional distance between two randomly chosen individuals (dbFD function in FD package, version 1.0-12, in R). i) **Rao's quadratic entropy** (using the abundance vector): measures mean functional distance between two randomly chosen individuals (dbFD function in FD package, version 1.0-12, in R). j) **Maximum distance in trait space** between strains. k) **Volume of trait space**: calculated by multiplication of eigenvalues of factor analysis. l) **Sum of squared length of minimum spanning tree in trait space** (SMST). m) **Area of MDS plot**: calculated by multiplication of the two first eigenvalues of factor analysis. n) **Standard deviation of interaction rates**. o) **Community population**: Number of Individuals in community. p) **Number of mass extinction events** over $5 \times 10^6$ generations. Each plot is the average of corresponding index over 3 simulations each over $5 \times 10^6$generations. Simulations are done with $\mu = 0.001$, $m = 0.02$ and $N_s = 10^5$.

## VII Cycles

Local flow of energy/mass in our community is determined by matrix $\boldsymbol{I}_{\alpha\beta} - \boldsymbol{I}_{\beta\alpha}$ which is an asymmetric matrix and its corresponding network is a directed network with one directed edge between each pair of nodes with weight between 0 and 1. We compare number and strength of cycles of this evolving network with its equivalent random networks. For this purpose we need

1. a method to find a cycle: We select 3 nodes of the network randomly and check if they form a cycle of size 3. If yes, it increases the number of cycles by 1 and the minimum weight of its edges would be assigned as its strength. This procedure is repeated many times ($> 10^5$) and then we average over the strengths.

2. to build random networks: We shuffle the edges of original network to obtain a random network. Then apply the procedure described in 1 on this network to measure the number of cycles and their strengths. This step is done several times ($> 10$) to have different random networks.

Result of these two steps are plotted in Fig. 1-g and Fig. 2-a in the paper.

## VIII Size of the system

Simulations with $N_s = 1 \times 10^4, 3 \times 10^4, 1 \times 10^5, 3 \times 10^5$, $\lambda = \infty$ and a set of trade-off parameters ($0 \leq \delta < 1$) were done to check the effect of size of the system. One of the diversity indexes (SMST) is plotted in Fig. 8 for different sizes. As it is clear by increasing $N_s$ the final diversity in trait space is higher and the drop in $\delta = 0.7$ is sharper which is typical of a phase transition.

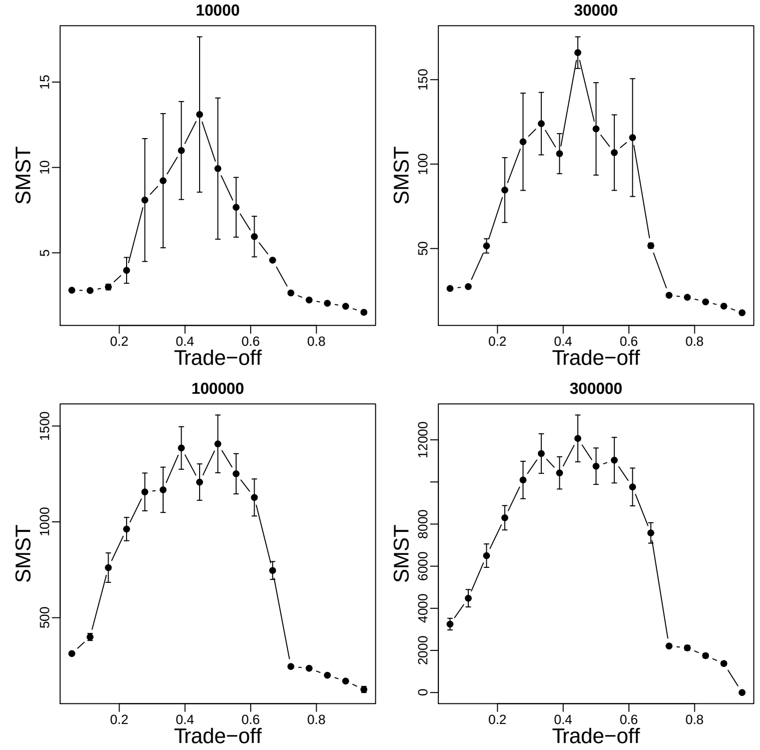


Figure 8: Functional diversity as measured by size of minimum spanning tree (SMST) as function trade-off parameter for different system sizes $N_s$. Simulations are done with $\lambda = \infty$, $\mu = 0.001$ and $m = 0.02$.

# IX Frequency-dependent selection

Frequency-dependent selection mediated by interaction of species could be a source for temporal correlation between eco-evolutionary events, e.g. speciation, invasion and extinction of species. To examine if there is such a correlation we used the distribution of inter-event times, i.e. distribution of intervals between occurrence of events. For a completely random process (Poisson process) this distribution follows an exponential distribution and deviation from exponential is a signature of correlation between events. Fig 9 shows inter-event distribution of ITEEM data and compares it with the best fit of geometric distribution (discrete version of exponential distribution) to data. The clear deviation from Poisson process shows that speciation and extinctions are not just random events but after occurrence of an event, with a delay ($\approx$ 10000 generations), the probability of observing a new event is higher than a random process.

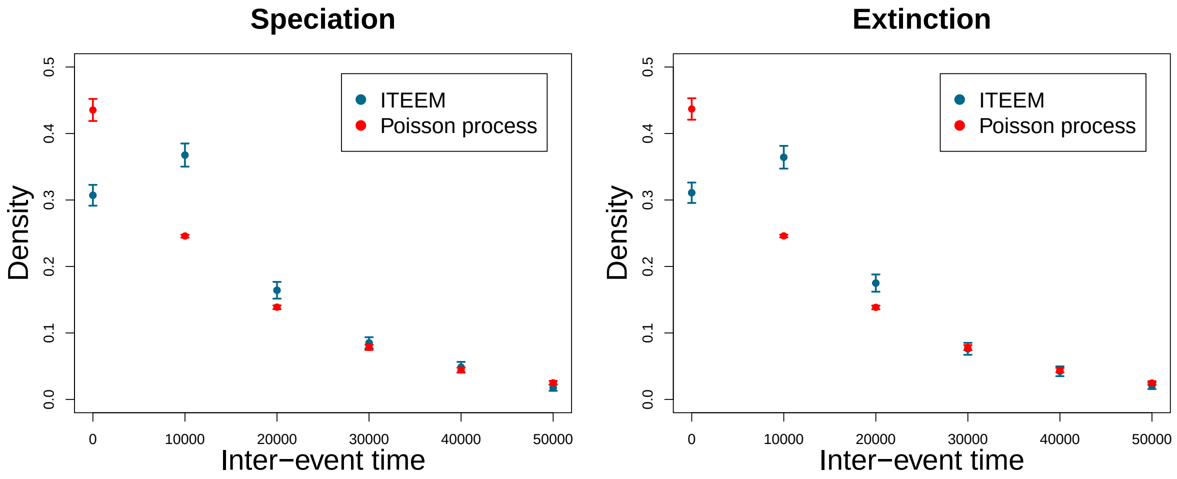


Figure 9: Distribution of time interval between speciation events (left) and extinction events (right). Blue points and error bars: data from 24 ITEEM simulations, each of $5 \cdot 10^6$ generations ($\delta = 0.5, \lambda = 10^5 \ldots \infty$, $N_S = 10^5$, $\mu = 0.001$, $m = 0.02$). Error bars are $\pm 2$ standard deviations calculated by bootstrapping. Red points and error bars: maximum likelihood fit (function fitdistr in R-package MASS, version 7.3-44) of the simulated data to a geometric distribution (discrete version of an exponential distribution), corresponding to an assumed Poisson process. Error bars are $\pm 2$ standard deviations estimated by the maximum likelihood fit.

# X Mutation Rate

Fig. 10 show behavior of typical diversity index (SMST) over $\delta$ and $\lambda$ for different mutation rates. Although the overall dependency on trade-off strength and lifespan is the same for a wide range of mutation rates but the size of diversity depends on mutation rate: the smaller the mutation rate the lower the diversity in community.

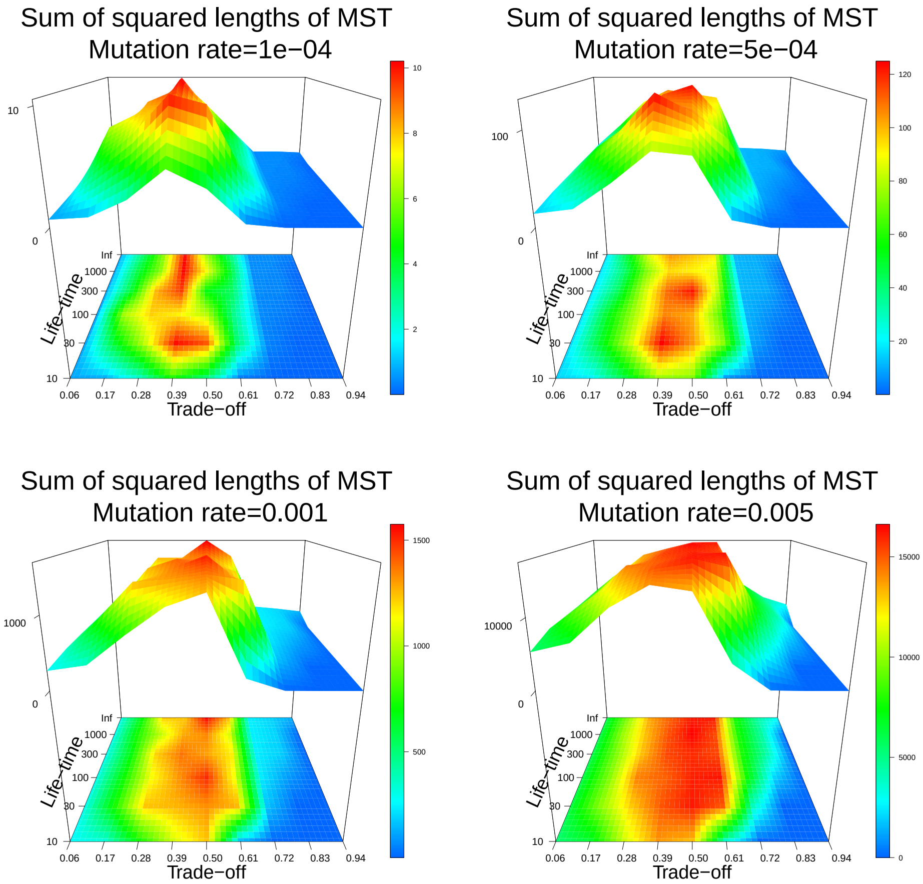


Figure 10: SMST for different mutation rates versus trade-off and lifespan.

Mutation rate also affects the rate of increase in diversity. Fig.11 shows the rate of increase in diversity (measured as increase of SMST per 10000 generations) for different mutation rates.

# XI Neutral Model

To compare the diversity generated by genetic drift (neutral model) with diversity generated under selection pressure induced by competition with moderate trade-offs, we do simulations in which all species compete equally for resources, i.e. $\boldsymbol{I}_{\alpha\beta} = 0.5$ for all species , but traits evolve by mutation as before. In the neutral model reproduction rates should also be the same for all species so we attribute the same reproduction rate in each simulation to all species. We carry out simulations for reproduction rates $r = 0.1$, $0.5$, $0.9$.

Distribution of strains over trait space (Fig. 12) show that genetic drift is able to spread trait vectors in trait space and produce cloud of strains but the size of diversity generated by it is much smaller than that of communities evolved under biotic selection pressure mediated by competition under moderate trade-offs.

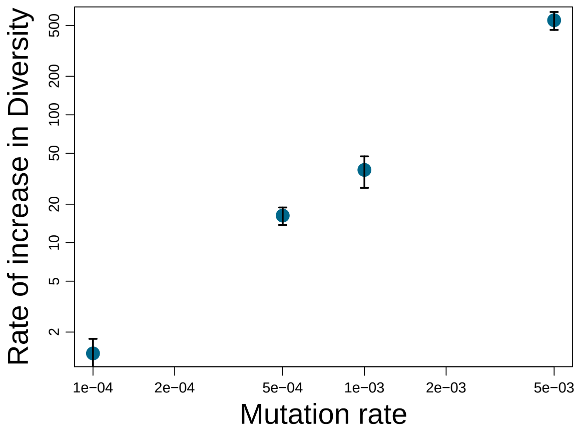


Figure 11: Rate of increase in diversity (measured as increase of SMST per 10000 generations) for different mutation rates. Rate of increase in diversity is calculated by fitting a line to the first 80000 generations of each simulation and averaging is over 5 different simulations. Error bars show the errors estimated by fit. Note the logarithmic scale of the plot.

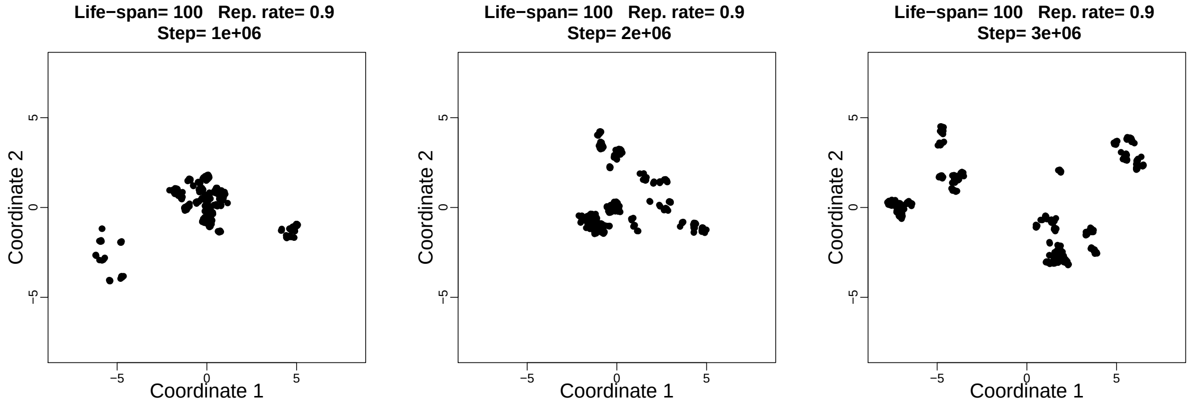


Figure 12: Trait space of a community evolved under neutral model in 3 time step: $1 \times 10^6$,$2 \times 10^6$ and $3 \times 10^6$ with $\lambda = 100$, $r = 0.9$, $\mu = 0.001$ and $m = 0.02$. Note the small size of the trait space in comparison to a no neutral model (SI Fig 3).

In order to show clearly the difference between the diversity produced in both models we also studied the diversity measures and other parameters. In Fig. 13, left panel in each row shows changes of a typical diversity index (SMST) over time for a simulation of genetic drift for one lifespan (with 3 different reproduction rates) and compares the results with a typical simulation with competitive selection pressure for a moderate trade-off ($\delta = 0.56$). Right panels illustrate the corresponding plots but for cycle formation. Relative strength of cycles in these simulations has big fluctuations around a value less than one, without any stable pattern over time. This shows that, as it is expected, dynamics of community in the neutral model is determined by fluctuations.

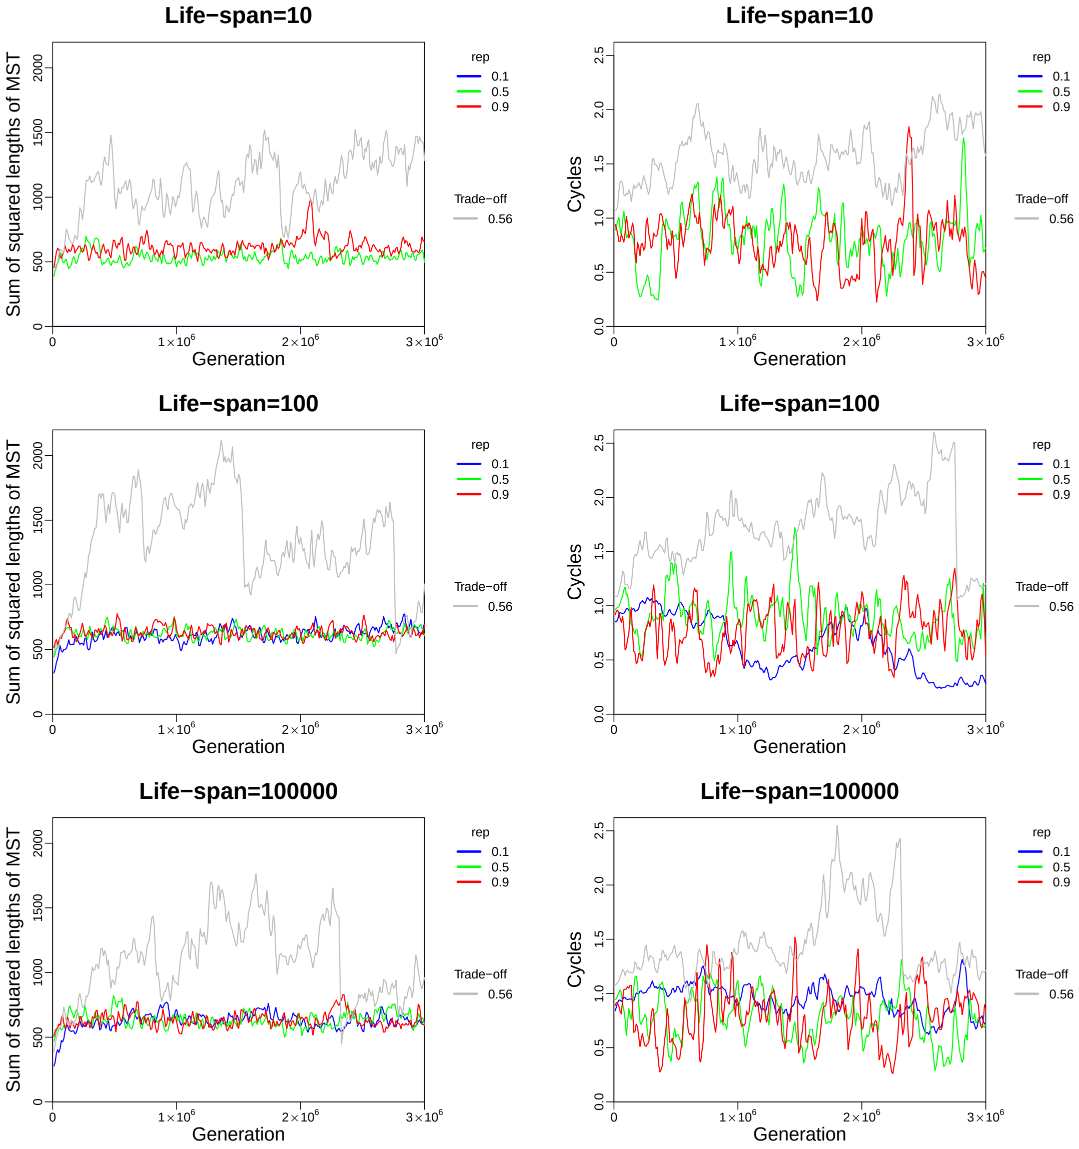


Figure 13: Plots in the left and right panels show how SMST and relative strength of cycles, respectively, change over generations for 3 different lifespans. Colored curves are the results of the neutral model with different reproduction rates ($r = 0.1, 0.5, 0, 9$). The results are compared with the outcome of one simulation with the corresponding lifespans and trade-off strength of 0.56 (gray curves). For $\lambda = 10$ and $r = 0.1$ population goes to extinction very fast.

# References

[1] Zachos, Frank E. "Introduction to the Species Problem." Species Concepts in Biology. Springer International Publishing, 2016. 1-16. (DOI 10.1007/978-3-319-44966-1_1)

[2] Pavlinov, Igor Ya. ”The Species Problem-Ongoing Issues” InTech, 2013. (DOI 10.5772/3313)

[3] Mouchet, M. A., Villéger, S., Mason, N. W. H., & Mouillot, D. “Functional diversity measures: An overview of their redundancy and their ability to discriminate community assembly rules. Functional Ecology, 24(4), 867–876, 2010. (10.1111/j.1365-2435.2010.01695.x)
